# Supplementary material for: New Physics at the TeV Scale
Source: arXiv:1604.07358 source file (2016-04-25)
Supplement: Supplementary file 1 [file appendix.tex]

\chapter{IMPORTANT TABLE}\label{chap:appA}
 Appendix~\ref{chap:appA} goes here.  Table~\ref{tbl:appA:table1} is copied from Chapter~\ref{chap:chap3}.
\begin{table}[h]
\caption{Sample multicolumn table}
\begin{center}
  \begin{tabular}{|l|cc|cc|}
    \hline
  Parameter & \multicolumn{2}{c|}{Column 1} & \multicolumn{2}{c|}{Column 2}\\ \cline{2-5}
              & Subcolumn 1 & Subcolumn 2 & Subcolumn 1 & Subcolumn 2 \\
\hline
    Parameter 1 & Element 11 & Element 12 & Element 13 & Element 14\\
    Parameter 2 & Element 21 & Element 22 & Element 23 & Element 24\\
    Parameter 3 & Element 31 & Element 32 & Element 33 & Element 34\\
    \hline
\end{tabular} \label{tbl:appA:table1}
\end{center}
\end{table}
\chapter{MORE DATA}\label{chap:appB}
Appendix~\ref{chap:appB} data goes here
